# Supplementary material for: Landau Level Single-Electron Pumping
Source: arXiv:2406.13615 ancillary file (2025-01-02)
Supplement: Supplementary file 1 [file Supplementary_Document.pdf]

### Evolution of Pumped Current as a Function of Magnetic Field

As part of the supplementary info we have made available two movies (Side.mp4 and Front.mp4 ) of our experimental data taken from our electron pumps in the dilution fridge. The entrance gate voltage, entrance gate RF frequency, RF amplitude and source-drain bias are fixed to the following values: -600mV, 180MHz, 300mV and 100 mV respectively, as detailed in the paper. The movies show evolution of the pumped electrons as the exit gate voltage is swept from -800mV to -3000mV for magnetic fields from 1T to 9T. Two different views are shown to emphasise the effect the magnetic field has on the formation of the quantised plateaus. The formation of the plateaus at resonance is clearly visible in both videos at 7.2T as well as the oscillatory behaviour of the plateau length and position as a function of magnetic field. This behaviour is correlated to the SdH oscillations as described in the paper. The images below are snap shots from the movies.

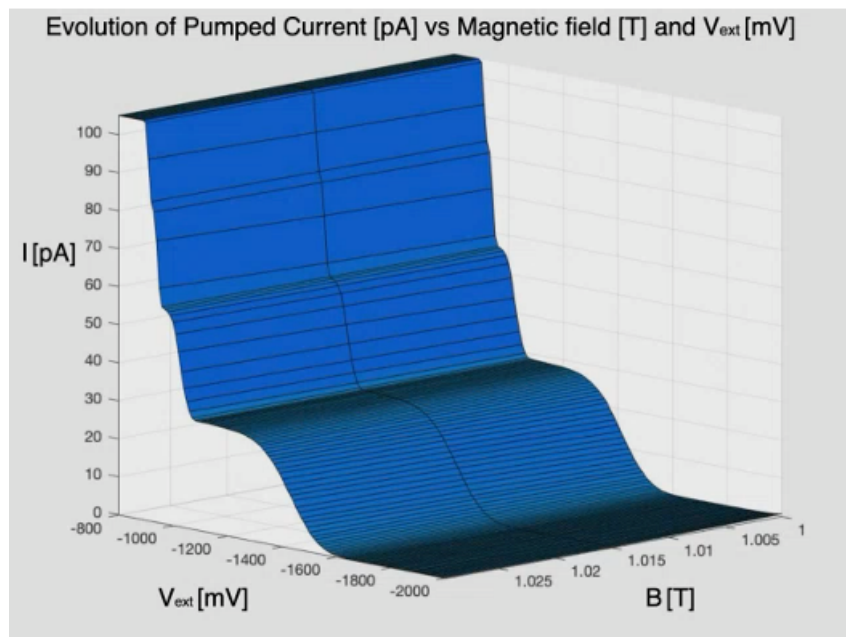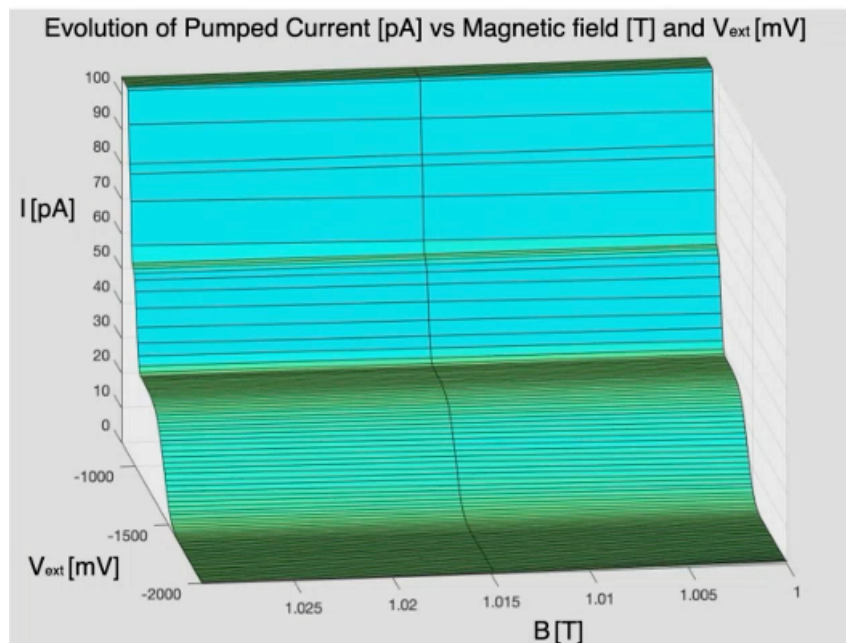

## Determination of Capture via Modelling of the Density of States Magnetic Field Dependency

As detailed in the paper under the data analysis section, simulation code written in Matlab was used to extract the capture energy of the pump based on the experimentally determined density of electrons  $n_D = 1.53 \times 10^{15} \text{ m}^{-2}$  and Landau broadening  $\Gamma = 1.35 \times 10^{-22} \text{ J}$ . Figure numbers given here in red refer to the figures in the paper, whilst figure numbers given in black refer to figures in this supplementary document.

$\Gamma$  as discussed in the paper was determined from the width of the resonance peak at 7.2T. This method was justified by the theoretical pump model presented in the paper. The strong correlation between the SdH oscillations and onset of pumping (Fig 1e), indicates that the pump's ability to transport quantised current is related to the density of states in the leads. The SdH analysis determined categorically that at around 6T the Fermi energy was pinned in the localised state with a filling factor of  $\nu = 2$ , including spin. The 7.2T resonance peak in the pumped data from its base on the left at 6T to its base on the right at 8.2T, is attributed to the capture energy of the pump relative to the first Landau level, where both the centre of the Landau level and the density of the level changes as a function of B. The resonance with its signature rise and fall allows us to define an evaluation point for the capture energy which we set to the centre of the first Landau level at 7.2T, as shown in Fig 4a. The form of the resonance peak indicates that the Landau level itself will move through this capture energy as the B field is stepped between 6T and 7.2T. If the capture energy of the pump at a specific B field is within the Landau level and less than or equal to the current value of the Fermi energy, capture will take place. We can consider two possible scenarios for the dynamics of the capture energy as a function of magnetic field.

1. The capture energy is fixed at the energy corresponding to the peak of the first Landau level at 7.2T for all magnetic field.
2. The capture energy at 7.2T corresponds to the energy of the centre of the first Landau level but then changes as a function of magnetic field monotonically for all magnetic fields.

We test each scenario in turn by plotting the density of states as a function of magnetic field for fixed capture energy as shown in Fig 4b (dashed turquoise line) and for a capture energy changing from  $E_c = 1.21 \times 10^{-21} \text{ J}$  to  $E_c = 1.60 \times 10^{-21} \text{ J}$  in step with the change in B from 1T to 9T, in multiples of  $\Delta B = 9.0 \times 10^{-4} \text{ J}$  as shown in Fig 4b (dark blue trace). In our simulation we consider the effect of accounting for spin and as is shown here, the inclusion of spin improves the correlation between the simulation and experimental data.

We present below a series of plots that were produced during our simulation that assisted in arriving at the final results presented in Fig 4.

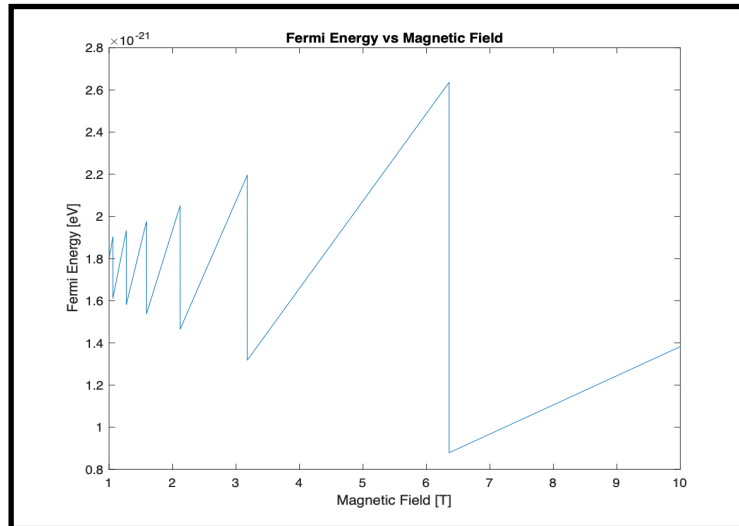

Figure 1

Figure 1 is that of the Fermi energy vs magnetic field, also known as the Fermi fan. Here one can observe how the Fermi energy changes as a function of magnetic field assuming a Landau broadening  $\Gamma = 0$  J and density of electrons  $n_D = 1.53 \times 10^{15} \text{ m}^{-2}$  and not taking into account spin.

If spin is considered the Fermi energy vs magnetic field is shown in Figure 2.

For completeness we report the change in Fermi energy as a function of magnetic field including the Landau

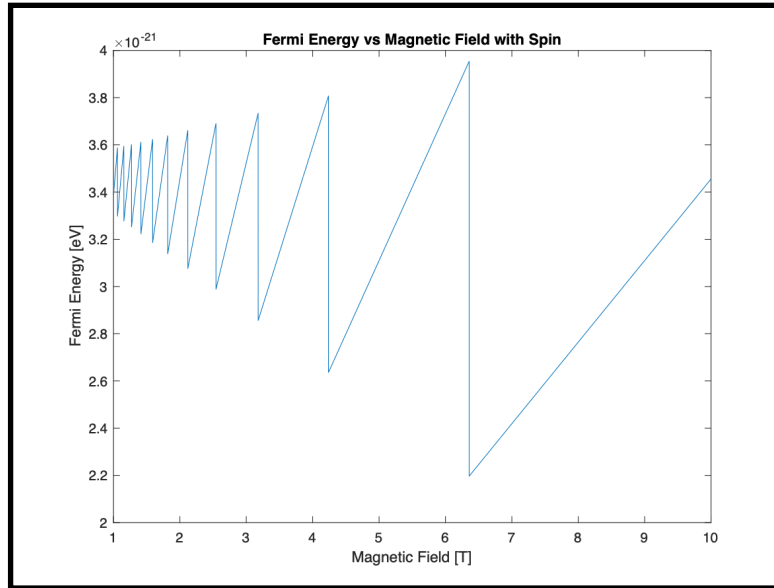

Figure 2

broadening  $\Gamma = 1.35 \times 10^{-22}$  J. We once again plot first with no spin (Figure 3) and then with spin (Figure 4).

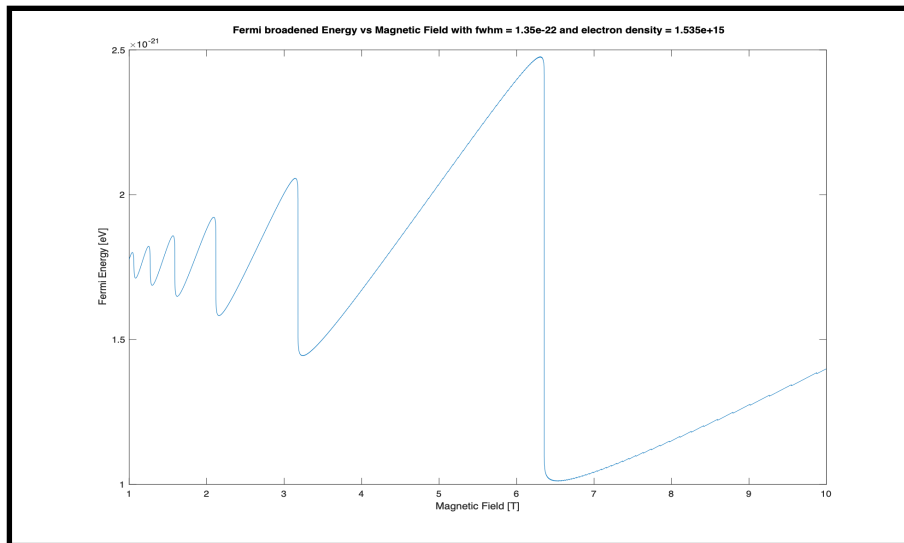

Figure 3

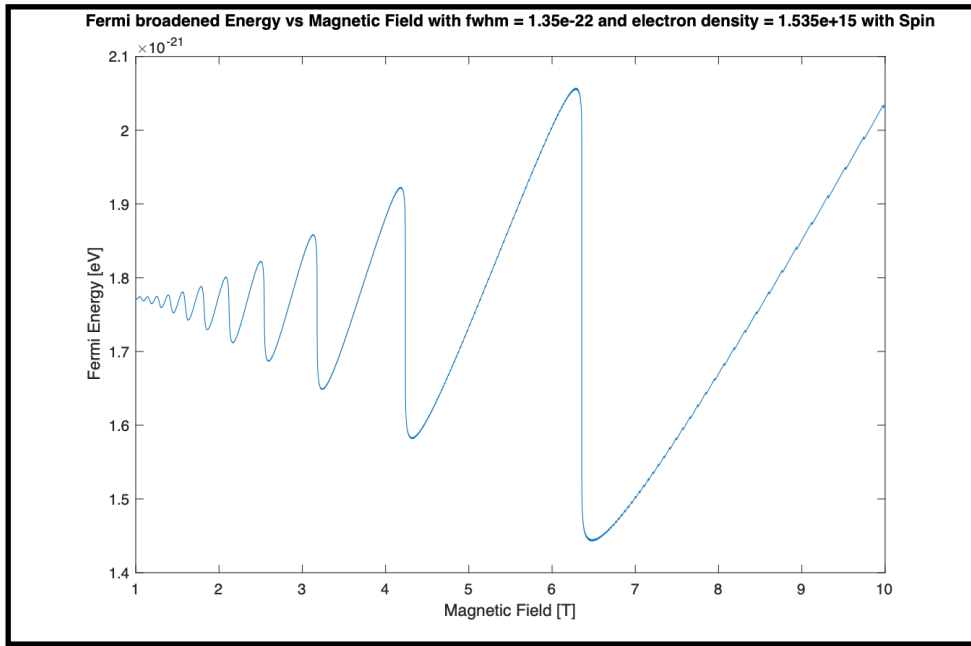

Figure 4

There is a clear difference in the Fermi energy evolution between Figures 1,2,3 and 4. If the capture energy is within a Landau level but above the Fermi level no capture will take place.

We next modelled how the Landau levels change as a function of magnetic field from  $B = 1\text{T}$  to  $10\text{T}$  in steps of  $1\text{T}$  and plot the evolution of the Fermi energy, shown in red as the Landau levels shift. First ignoring spin (Figure 5 – 6) and then with the inclusion of spin (Figure 7 - 8).

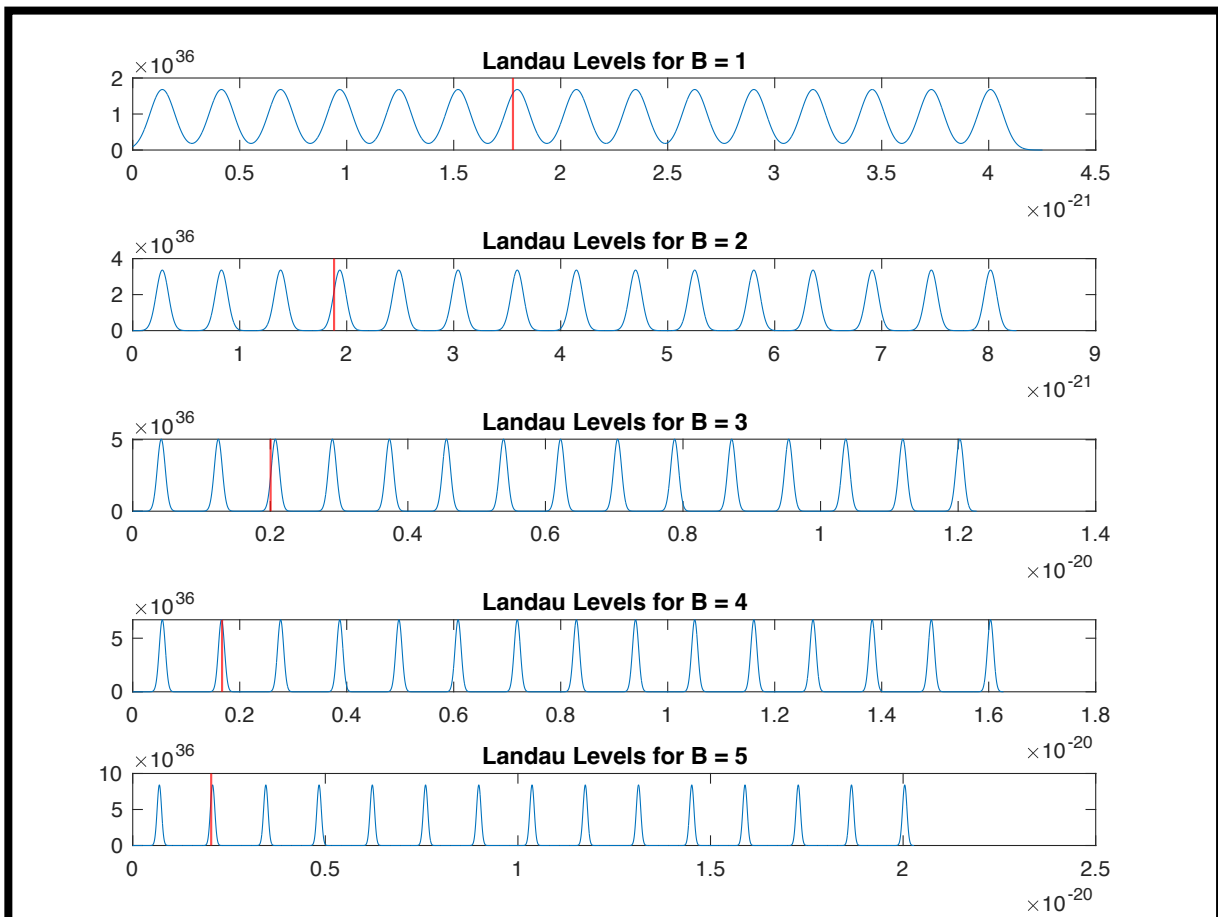

Figure 5

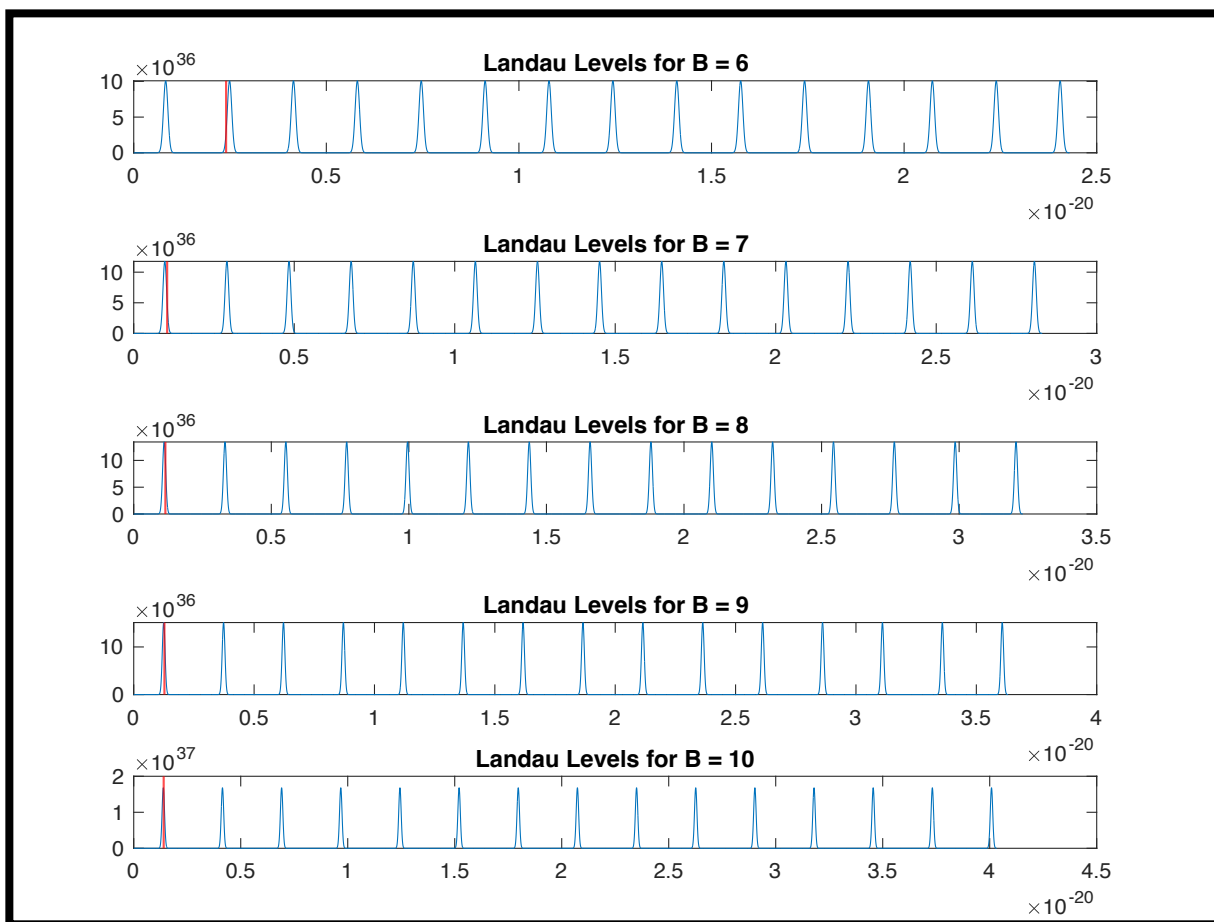

Figure 6

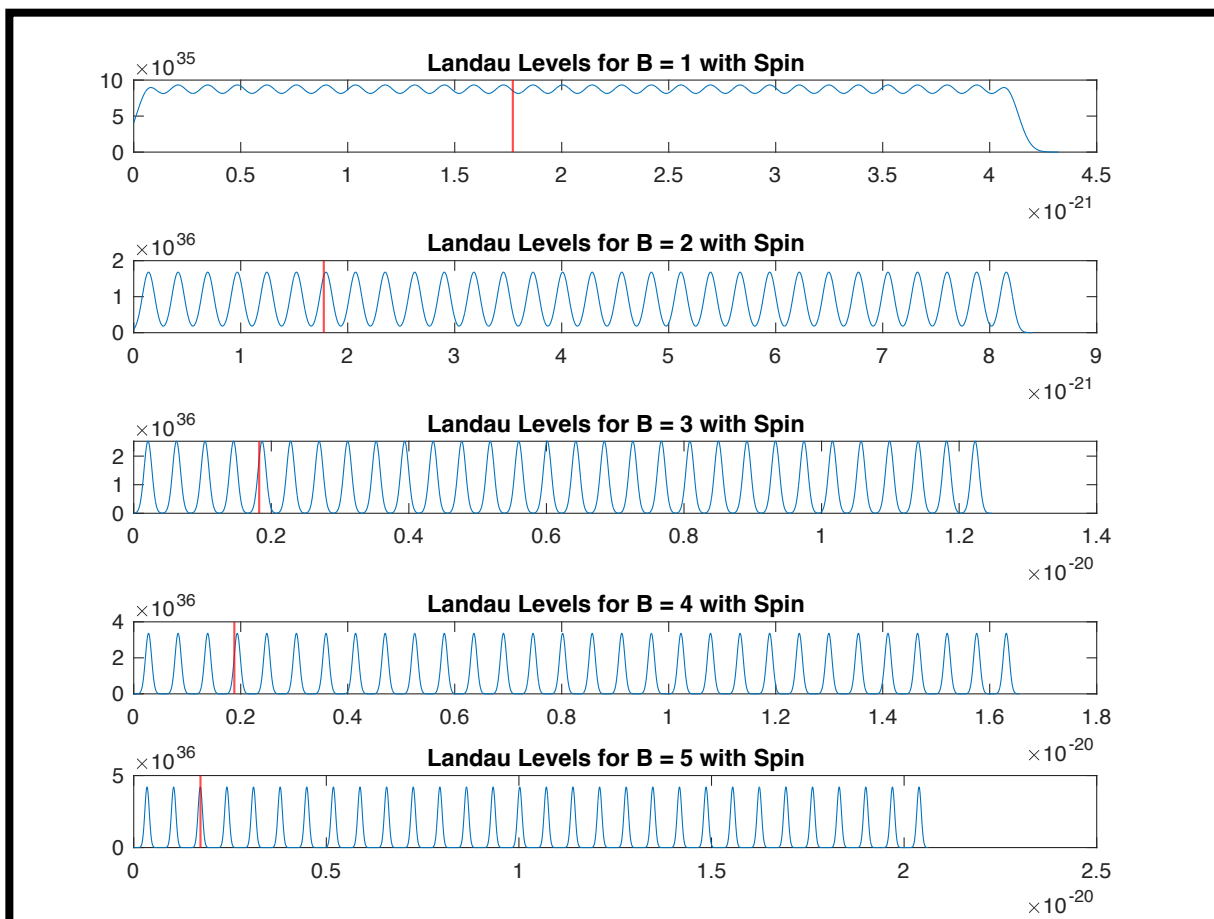

Figure 7

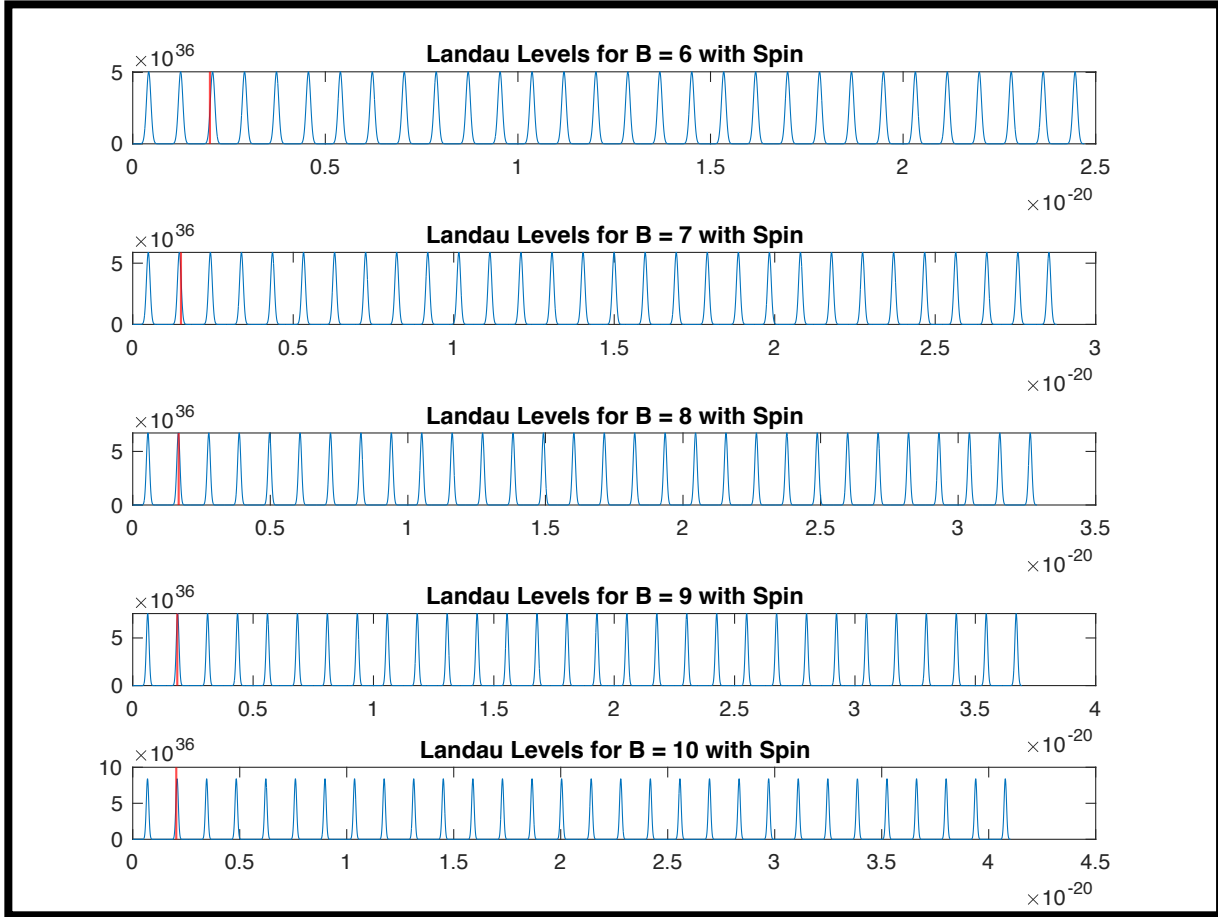

Figure 8

The movement of the Fermi energy in each plot shown in red, takes in to account the changing Landau level as well as density of each Landau level as the B field is changed.

The reader should note that different scales are used on both the x-axis and y-axis across all the above plots. In all plots we made use of the determined Landau broadening  $\Gamma = 1.35 \times 10^{-22}$  J as detailed in the paper and the determined density of electrons  $n_D = 1.53 \times 10^{15} \text{m}^{-2}$ .

Figure 9 -10 is the density of states vs magnetic field for a fixed capture energy during the full B sweep. Figure 9 shows with no spin consideration and Figure 10 with spin. A clear difference is seen with spin inclusion. With the spin there is far stronger correlation to the pumped data as shown in [Fig 4b](#)). Figure 10 shown here is plotted as the turquoise dotted plot in [Fig 4b](#)).

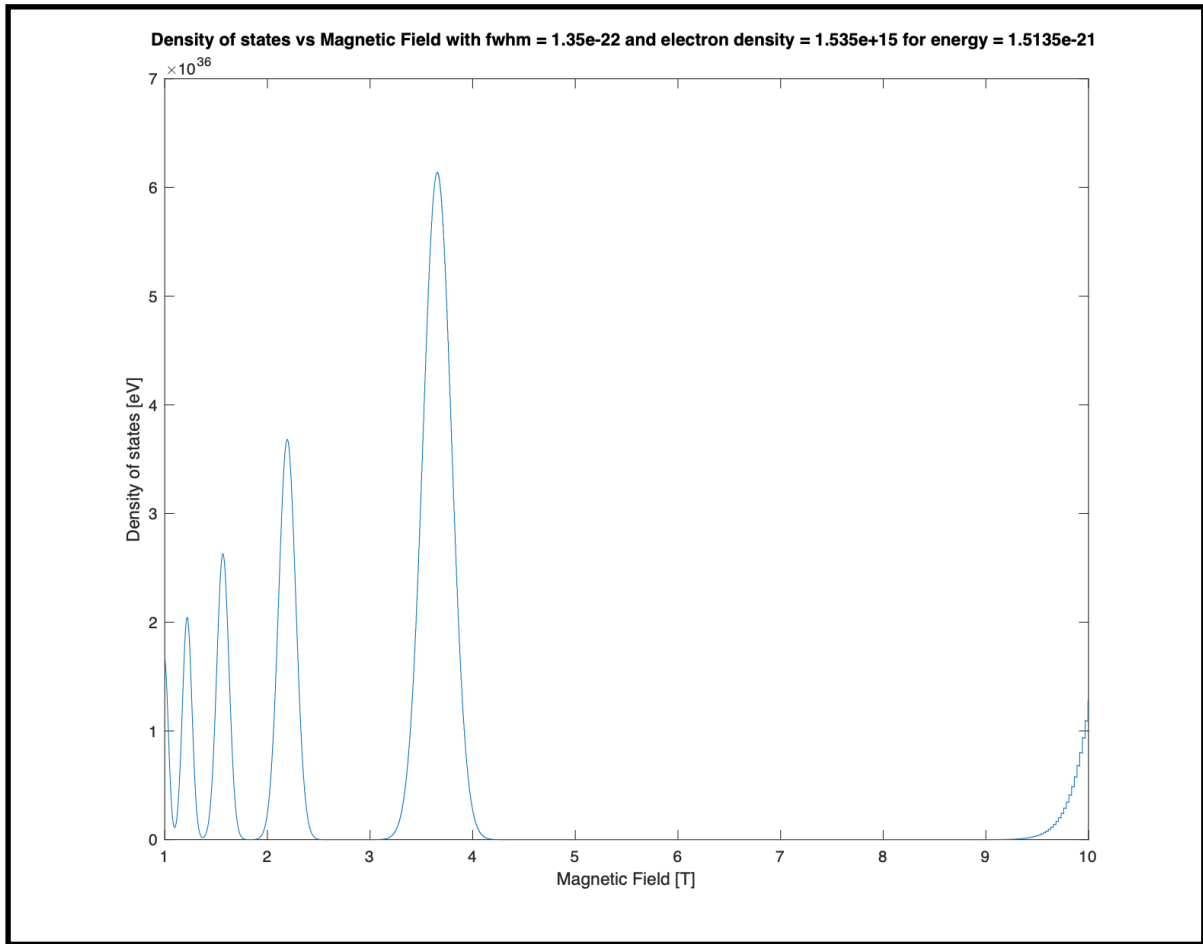

Figure 9

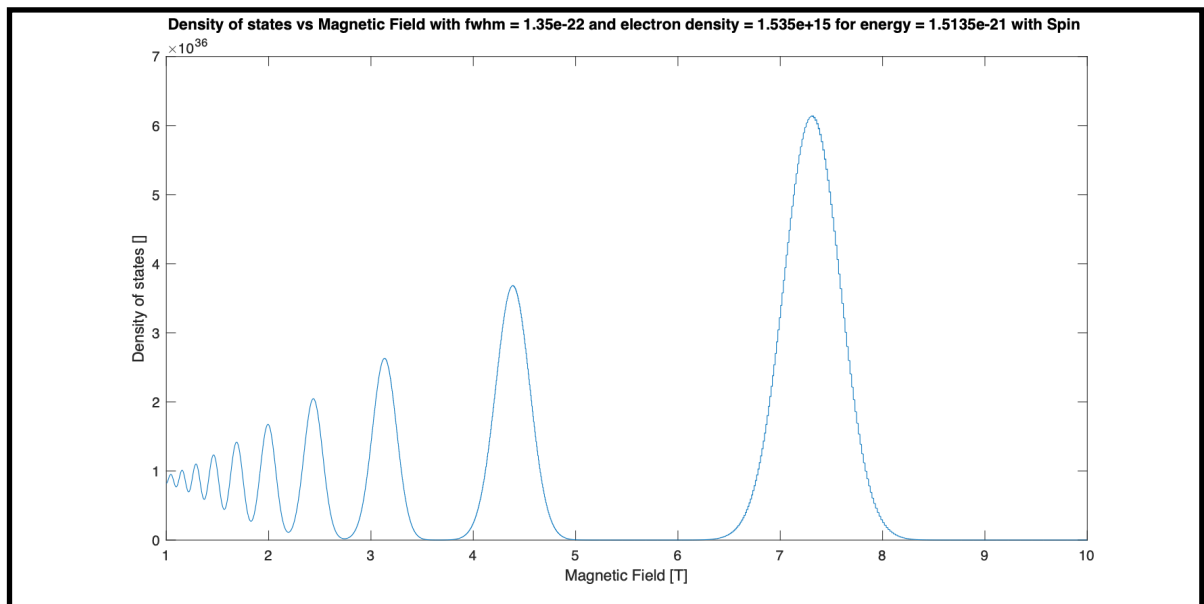

Figure 10

Figure 11 shows the density of states vs magnetic field for a changing capture energy during the full B sweep. In Figure 11, no spin considerations were made.

In Figure 12, spin was included. This plot therefore included a changing capture energy as the B field is swept and the inclusion of spin. It was plotted in Fig4b) as the dark plot line plot and corresponds very well with the red onset line of pumped current.

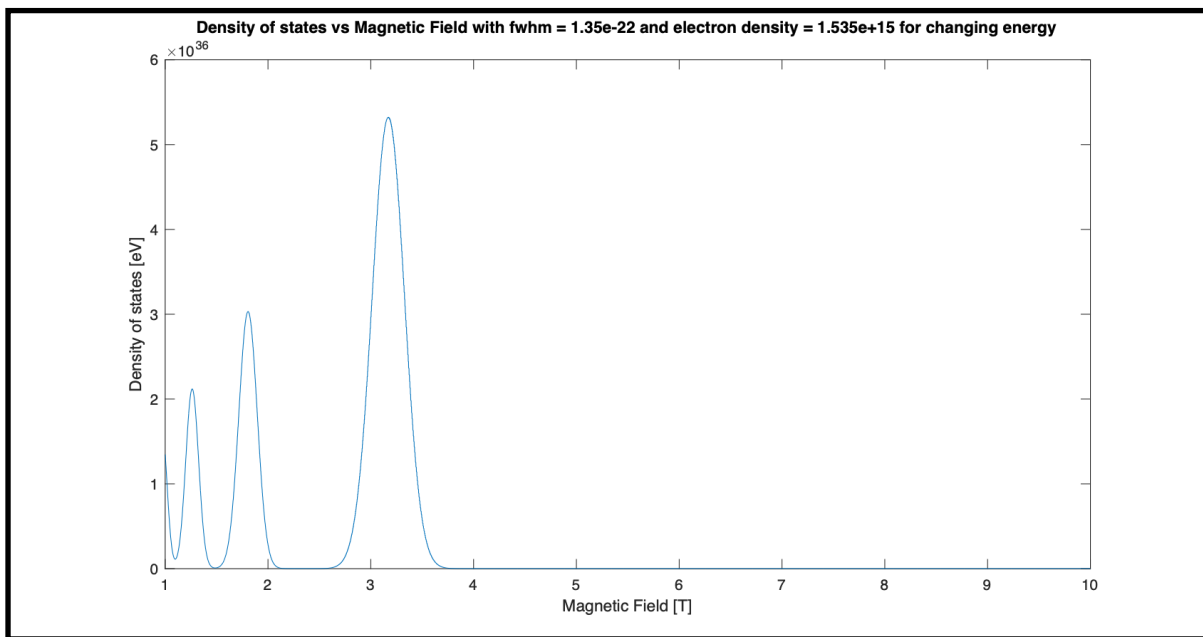

Figure 11

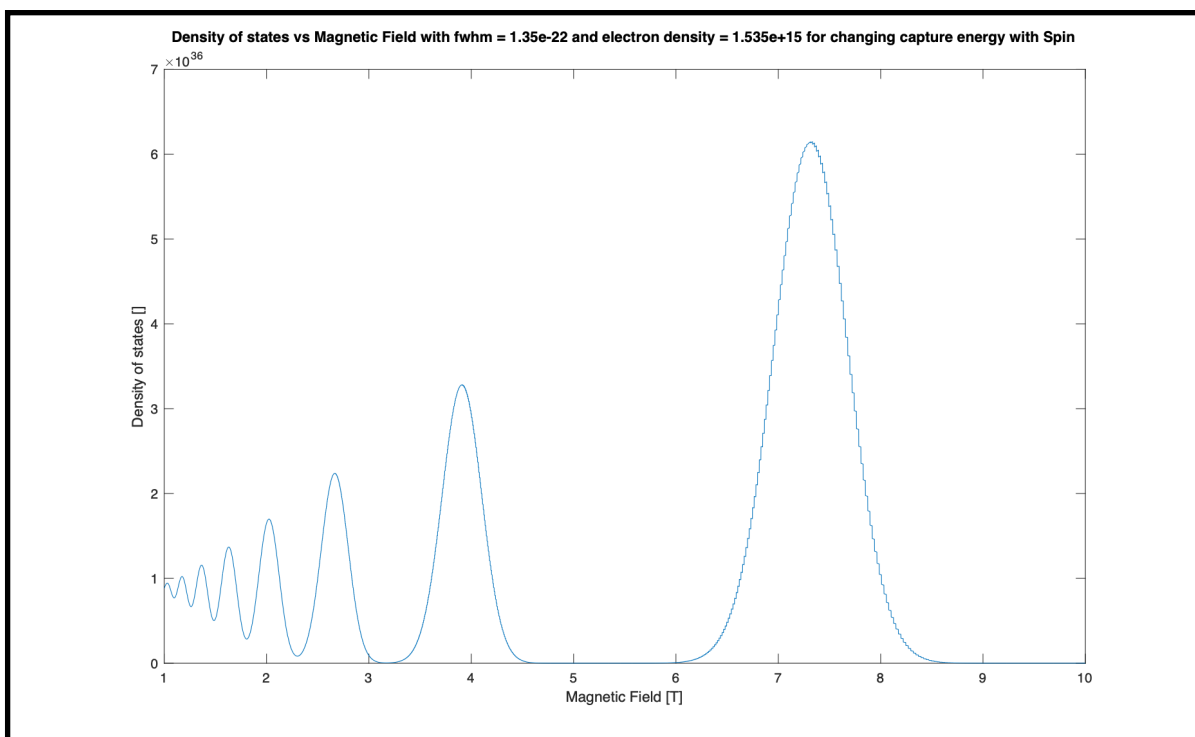

Figure 12
